# Supplementary material for: Low disorder and high valley splitting in silicon
Source: arXiv:2309.02832 ancillary file (2024-02-02)
Supplement: Supplementary file 1 [file Degli_Esposti_Supplementary.pdf]

# Supplementary Information: Low disorder and high valley splitting in silicon

Davide Degli Esposti,[1] Lucas E. A. Stehouwer,[1] Önder Gül,[2] Nodar Samkharadze,[2] Corentin Déprez,[1] Marcel Meyer,[1] Ilja N. Meijer,[1] Larysa Tryputen,[2] Saurabh Karwal,[2] Marc Botifoll,[3] Jordi Arbiol,[3,4] Sergey V. Amitonov,[2] Lieven M.K. Vandersypen,[1] Amir Sammak,[2] Menno Veldhorst,[1] and Giordano Scappucci[1,*]

[1] *QuTech and Kavli Institute of Nanoscience, Delft University of Technology, Lorentzweg 1, 2628 CJ Delft, The Netherlands*
[2] *QuTech and Netherlands Organization for Applied Scientific Research (TNO), Stieltjesweg 1, 2628 CK Delft, The Netherlands*
[3] *Catalan Institute of Nanoscience and Nanotechnology (ICN2), CSIC and BIST, Campus UAB, Bellaterra, 08193 Barcelona, Catalonia, Spain*
[4] *ICREA, Pg. Lluís Companys 23, 08010 Barcelona, Catalonia, Spain*

(Dated: February 1, 2024)

## CONTENTS

1. Measurement of the thickness and sharpness of the quantum wells 2

2. Strain analysis with Raman spectroscopy 4

3. Supplementary mobility density curves 5

4. Charge noise measurements 6

5. Valley splitting measurements 9

References 10

[*] g.scappucci@tudelft.nl

## 1. MEASUREMENT OF THE THICKNESS AND SHARPNESS OF THE QUANTUM WELLS

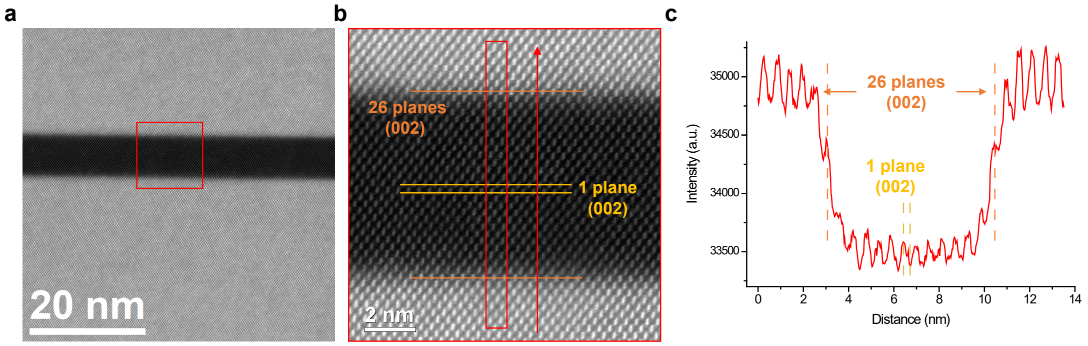


Figure S1. Method for computing the thickness of the quantum well based on the counting of the (002) horizontal planes, which reduces the uncertainty and bias associated with properly detecting the margins of the quantum well.

We measure the thickness of the Si layer quantum well ($w$) by considering the interplanar spacing of the horizontal planes (002) of the quantum well ($d_{qw}$) and of the underlying strain-relaxed SiGe buffer layer ($d_{buffer}$). For the $Si_{1-x}Ge_x$ buffer layer, we consider the stoichiometry $x = 0.31(1)$ as measured by means of quantitative EELS and SIMS[1, 2] and calculate the expected cell parameter $a_{cell}$ using the following approximation of Vegard's law[3]:

$$a_{cell} = \ a_{Si} + 0.20x + 0.027x^2 = 2.75(9) \text{ Å} \tag{S1}$$

where $a_{Si} = 5.431$ Å bulk Si lattice constant, and $x = 0.31(1)$. To calculate $d_{buff}$, we use the formula for the interplanar distance of the (002) plane in a diamond cubic system:

$$d_{hkl} = \frac{a_{cell}}{\sqrt{h^2 + k^2 + l^2}} \ = \ \frac{a_{cell}}{\sqrt{0^2 + 0^2 + 2^2}} \ = \ \frac{a_{cell}}{2}. \tag{S2}$$

Since the quantum well is strained, $d_{qw}$ is found by considering the average dilatation $\delta$ of the quantum well (002) planes with respect to the (002) planes of the buffer. The dilatation $\delta$ is measured by Geometrical Phase Analysis (GPA). The standard deviation of GPA is high for dilatation close to 0, as happens with the (220) epitaxial planes, for which the method is not the preferred choice. Nevertheless, for the larger dilatation of the (002) planes, the relatively smaller standard deviation makes the measurement significant. As a result, $d_{qw}$ is computed by:

$$d_{qw} = \ d_{buff}\,(1 + \delta)\,. \tag{S3}$$

Finally, the thickness of the quantum well is given by:

$$w = n_{qw} d_{qw}, \tag{S4}$$

where $n_{qw}$ is the number of atomic planes in the (002) direction forming the quantum well, and $d_{qw}$ is the distance between two planes. Therefore, the expected uncertainty of the thickness measurement lies in whether the initial and last plane of the well is being considered or not, *i.e.*, the standard deviation is given by $\sigma = 2d_{qw}$.

We perform four different measurements and count the (002) planes in different regions of the quantum well. We find $n_{qw} = 25$ two times, and $n_{qw} = 26$ two times. We measure an average $\delta = -1.700 \pm 0.003$ of %, leading to $d_{qw} = 2.70 \pm 0.01$ Å, and resulting in an average thickness $w = 6.9 \pm 0.5$ nm.

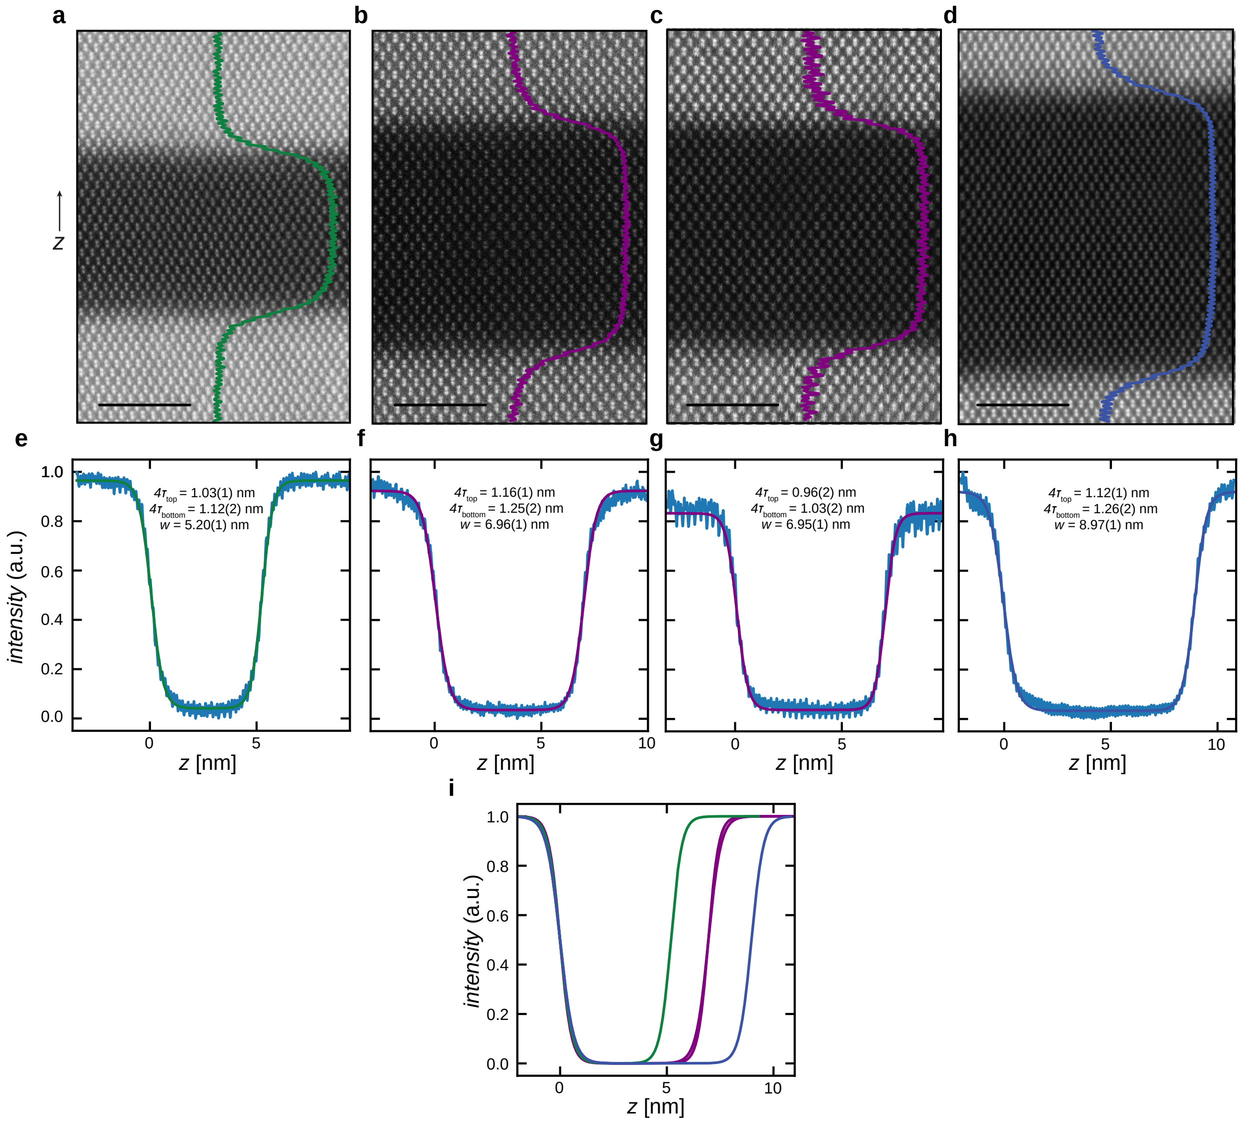


Figure S2. **a-d** High-resolution STEM with superimposed intensity profiles from multiple wafers featuring different thicknesses of the quantum well. All images are taken on wafers featuring the H-FET gate stack, *i.e.*, where the first steps of the fabrication process have been executed to resemble the condition of the actual quantum dot devices. The black scale in all images corresponds to 3 nm. Images in **b** and **c** come from two nominally identical heterostructures, *i.e.* grown using the same recipe on two wafers. **e-h** Corresponding intensity profile from **a-d** with superimposed fit to a sigmoid function as reported in Eq. S5. From this fit, we extract the parameters characterizing the sharpness of the bottom ($\tau_{bottom}$) and top ($\tau_{top}$) interfaces, and the quantum well thickness ($w = x_{top} - x_{bottom}$). **i** Comparison of the fitted sigmoid intensity profiles for the three heterostructures considered in the main text featuring quantum wells that are nominally 5 nm, 7 nm, and 9 nm wide

We validate the thickness of the quantum well ($w$) and quantify the sharpness of the top and bottom interfaces by fitting the intensity profile with a Sigmoid function[4]:

$$I(x) = \frac{1}{1 + e^{\frac{x_{top} - x}{\tau_{top}}}} + \frac{1}{1 + e^{\frac{x - x_{bottom}}{\tau_{bottom}}}} \tag{S5}$$

where $x_{top}$ and $x_{bottom}$ are the position of the top and bottom interfaces, and $\tau_{top}$ and $\tau_{bottom}$ are the characteristic length quantifying the top and bottom interfaces of the quantum well, *i.e.*, the SiGe/Si and Si/SiGe interfaces. We characterize the interface sharpness with the $4\tau$ parameter corresponding to the length over which the intensity profile changes from 0.12 to 0.88 of the asymptotic value.

## 2. STRAIN ANALYSIS WITH RAMAN SPECTROSCOPY

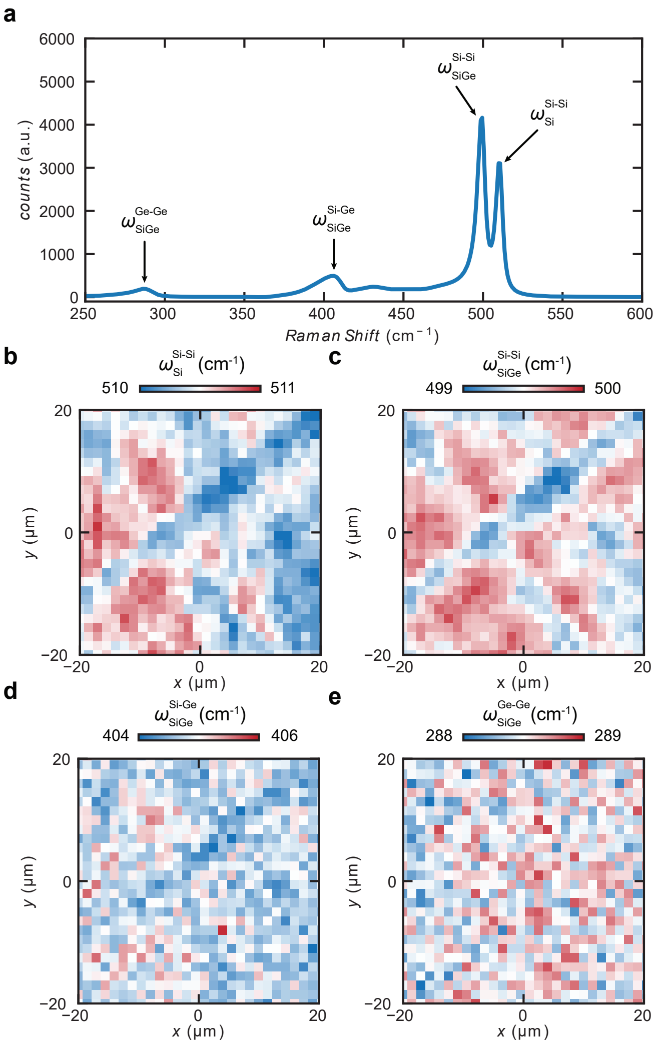


Figure S3. **a** Typical Raman spectrum of a Si/SiGe heterostructure without the SiGe topmost barrier acquired using a violet laser. The spectrum shows multiple peaks corresponding to the Si-Si vibration in the Si quantum well ($\omega_{\mathrm{Si}}^{\text{Si-Si}}$), and the Si-Ge, Si-Si, and Ge-Ge vibrations in the SiGe SRB ($\omega_{\mathrm{SiGe}}^{\text{Si-Ge}}$, $\omega_{\mathrm{SiGe}}^{\text{Si-Si}}$, and $\omega_{\mathrm{SiGe}}^{\text{Ge-Ge}}$, respectively). **b-e** 2D Raman mapping on a 40 μm of the various vibrations from the strained Si quantum well and virtual substrate. We find the average Raman shifts of these vibrations to be: $\overline{\omega}_{\mathrm{Si}}^{\text{Si-Si}} = 510.4(2)$ cm$^{-1}$, $\overline{\omega}_{\mathrm{SiGe}}^{\text{Si-Si}} = 499.5(2))$ cm$^{-1}$, $\overline{\omega}_{\mathrm{SiGe}}^{\text{Si-Ge}} = 404.8(3)$ cm$^{-1}$, and $\overline{\omega}_{\mathrm{SiGe}}^{\text{Ge-Ge}} = 288.5(5)$ cm$^{-1}$.

We calculate the strain of the Si quantum wells by converting phonon frequency shifts into strain[5, 6]:

$$\epsilon = \frac{\omega(\epsilon) - \omega_0}{b^{Si}}, \tag{S6}$$

where $\omega_0 = 520.7$ cm$^{-1}$ is the Raman shift associated with the Si-Si vibration from the unstrained Si substrate used to calibrate the Raman spectrometer, $b^{Si} = 784 \pm 4$ cm$^{-1}$ is the strain-shift coefficient for Si reported in ref. [7], and $\omega(\epsilon)$ is the Raman shift associated with the Si-Si vibration from the strained quantum well.

We calculate the expected strain ($\epsilon$) of the Si quantum well as:

$$\epsilon = (a_{SiGe} - a_{Si})/a_{Si} = 1.19(4)\% \tag{S7}$$

where $a_{SiGe}$ is calculated from Eq. S1 where $x = 0.31(1)$ is the Ge concentration in the SiGe buffer and spacer, and $a_{Si} = 0.5431$ nm is the lattice constant of bulk Si.

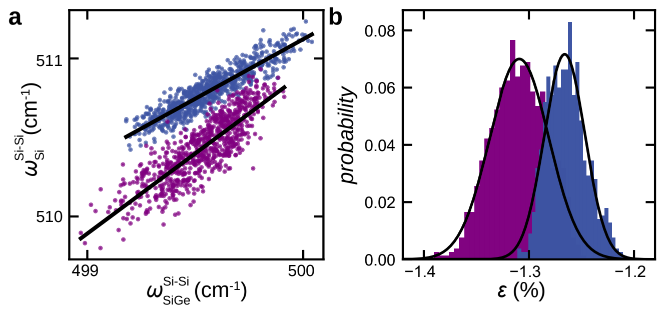


Figure S4. **a** Comparative cross-correlation plot of the Si-Si vibration from the strained Si quantum well ($\omega_{Si}$) and from the SiGe relaxed buffer ($\omega_{SiGe}$) for a quantum well with a thickness of 6.9(5) nm (purple) and 9.0(5) nm (blue). The black line is a linear fit to the data with an angular coefficient $a = 1.01(1)$ for the thinner well and $a = 0.75(2)$ for the thicker well. **b** Strain distributions for the two Si quantum wells. We find an average strain of $\bar{\epsilon} = -1.31(3)$ % for the 6.9(5) nm quantum well, and $\bar{\epsilon} = -1.26(2)$ % for the 9.0(5) nm quantum well.

## 3. SUPPLEMENTARY MOBILITY DENSITY CURVES

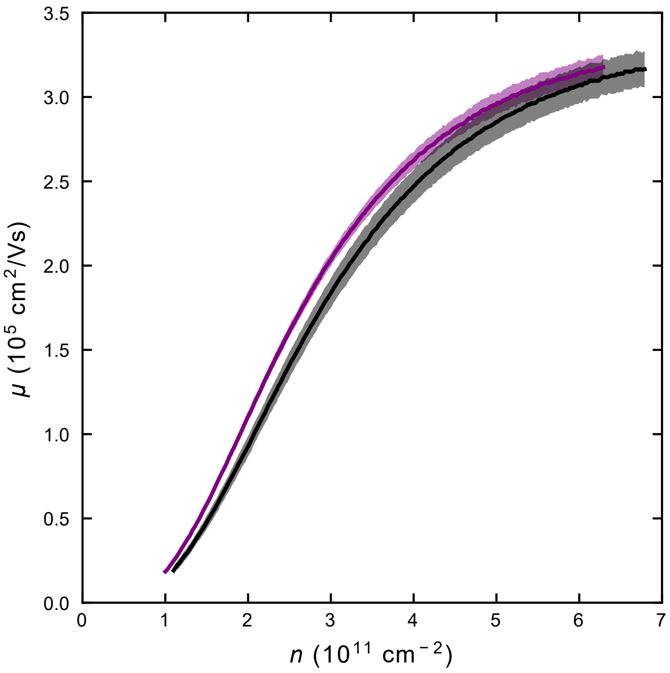


Figure S5. Mean mobility $\mu$ as a function of density $n$ measured at $T = 1.7$ K for H-FET coming from two different wafers grown using the same recipe at a distance of six months. Purple shows the data from the wafer SQ22-22-3 (10 HFET), and black shows data from SQ21-160-6 (10 HFET). The average mobility at a fixed density (solid line) and one standard deviation (shaded region) are shown.

## 4. CHARGE NOISE MEASUREMENTS

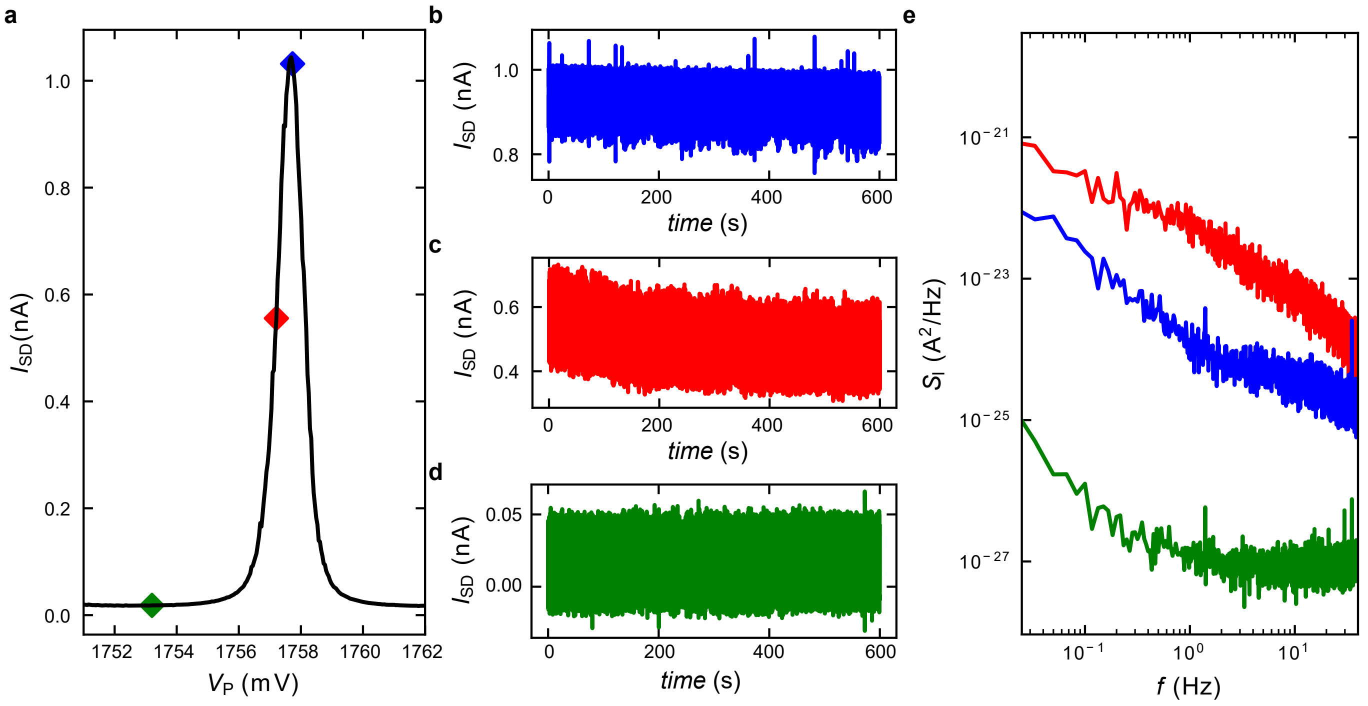


Figure S6. **a** Current ($I_{SD}$) as a function of plunger voltage ($V_P$) through one of the sensing dots tuned in the single electron regime. The top (blue), flank (red), and blockade (green) are highlighted with diamonds. **b-d** Current time traces in the three different configurations. We acquire ten minutes long time traces at a sampling rate of 1kHz. **e** Current noise power spectral density ($S_I$). $S_I$ is calculated by dividing the time traces into 10 segments of equal length, using the Fourier transform to convert to the frequency domain, and averaging the ten different Fourier transforms before calculating the power spectral density. As expected, we find that the noise measured at the flank of the Coulomb peak is the greatest [8].

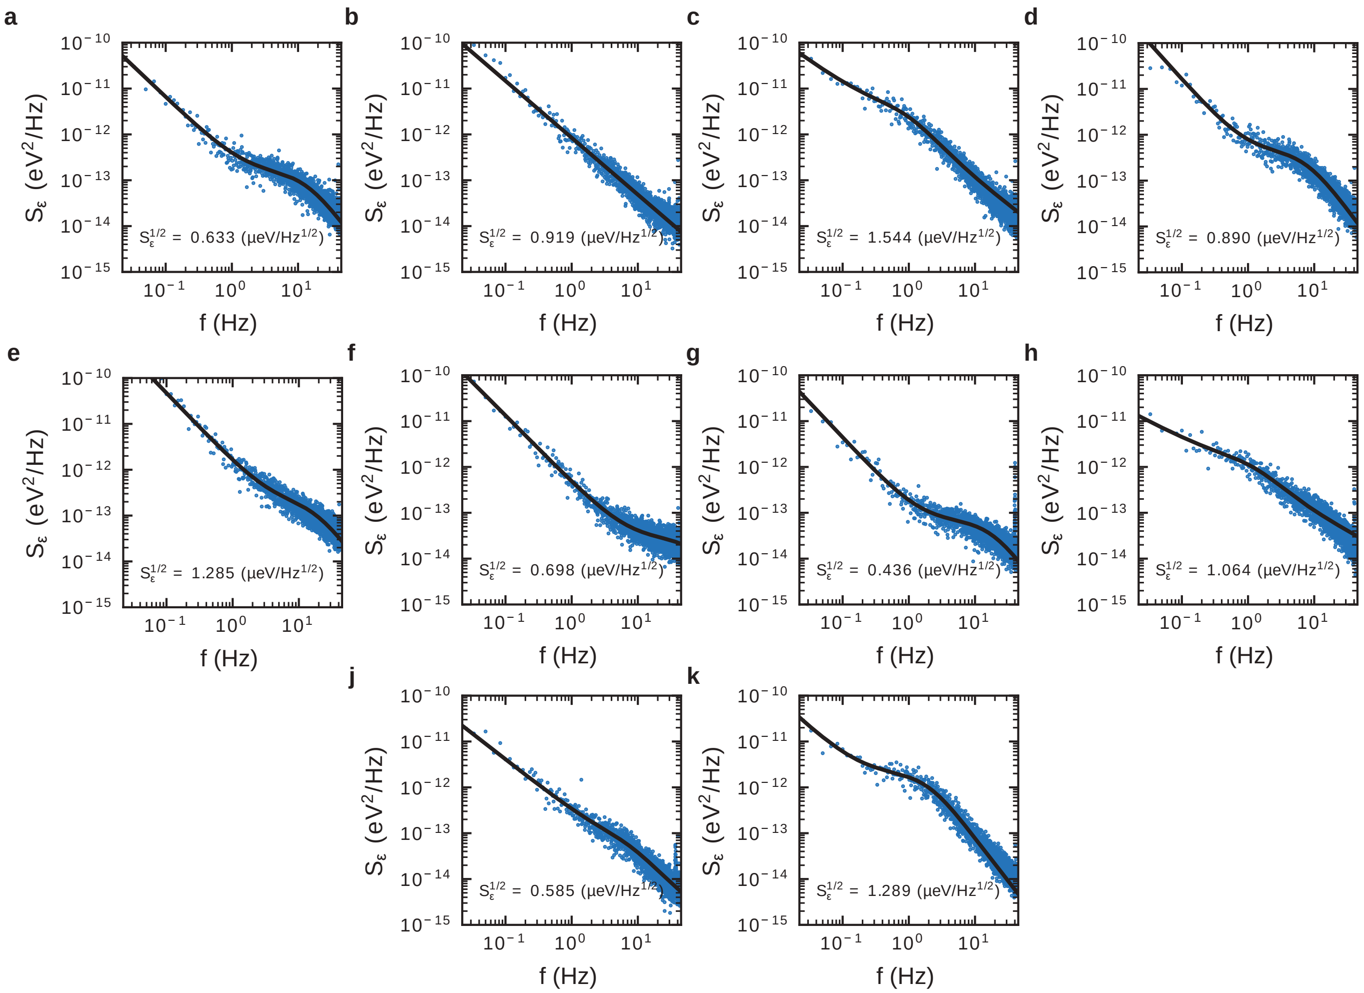


Figure S7. Charge noise power spectral density ($S_\epsilon(f)$) measured on a flank of a Coulomb peak and extracted using the lever arm of the corresponding Coulomb diamond for device A. The black line is a fit to the function which is the sum of a power law and a Lorentzian from which we extract the power spectral density at 1 Hz ($S_\epsilon^{1/2}$). The plots are arranged from **a** to **k** for increasing voltage applied to the sensor plunger.

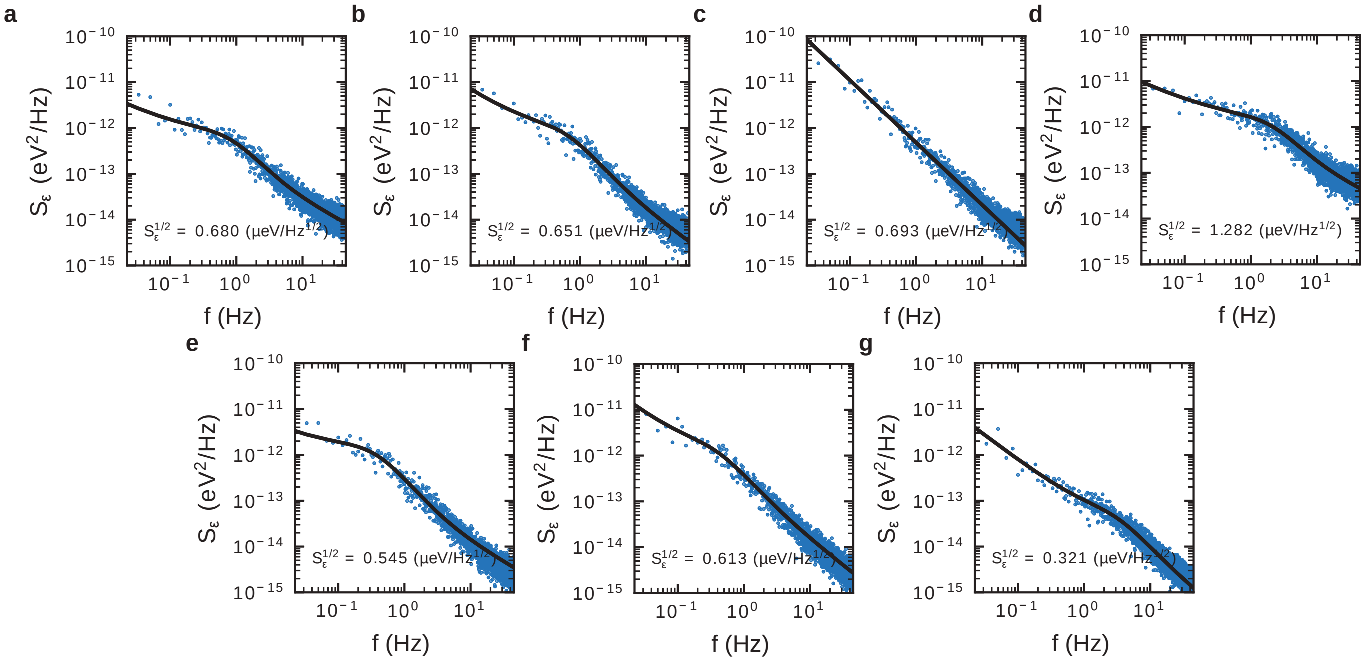


Figure S8. Charge noise power spectral density ($S_\epsilon(f)$) measured on a flank of a Coulomb peak and extracted using the lever arm of the corresponding Coulomb diamond for device B. The black line is a fit to the function which is the sum of a power law and a Lorentzian from which we extract the power spectral density at 1 Hz ($S_\epsilon^{1/2}$). The plots are arranged from **a** to **g** for increasing voltage applied to the plunger.

## 5. VALLEY SPLITTING MEASUREMENTS

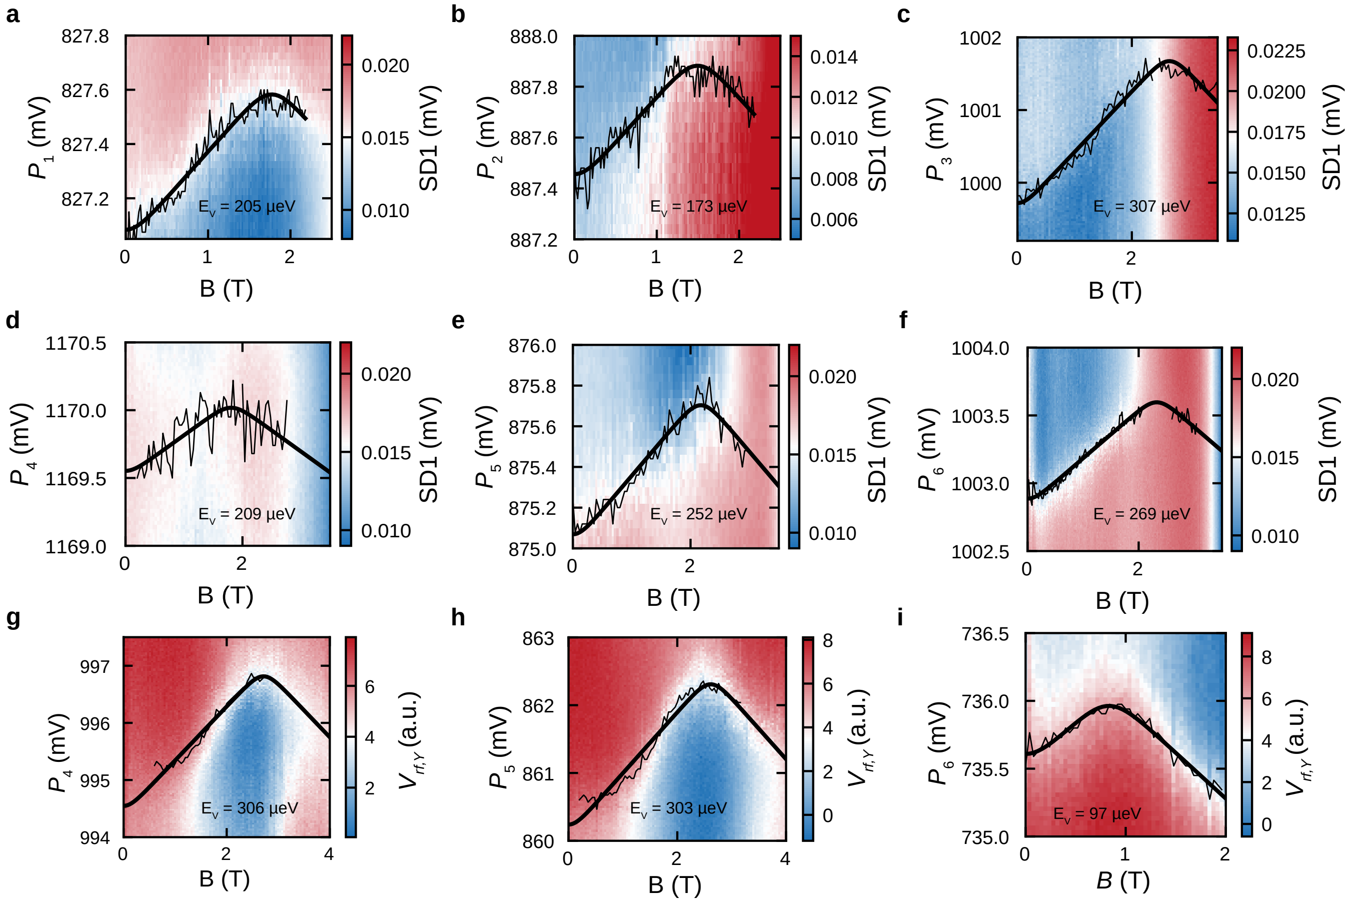


Figure S9. Magnetospectroscopy measurements of the 1e → 2e transition for Device 1 (six dots, **a**-**f**) and Device 2 (three dots, **g**-**i**). The thin black line follows the charge transition at a fixed magnetic field. We fit the evolution of the charge transition to the theoretical formula from ref.[2, 9] (thick black line). For $B = B_{ST}$, the Zeeman energy ($E_Z = -e\mu_B B$) equals the single-triplet splitting energy, and the typical kink can be observed.

We perform a Welch test[10] on the valley splitting measurements reported in Fig. 5b of the main text to quantify the statistical significance of our data. The Welch test is used to test the hypothesis that two populations with different variances have equal means. We obtain a $t$-value of 3.05 corresponding to a $p$-value of 0.78%, indicating that the probability that the measured data comes from distributions with the same mean is lower than 1 %. This confirms that our improvement in mean valley splitting has statistical significance.

[1] X. Xue, M. Russ, N. Samkharadze, B. Undseth, A. Sammak, G. Scappucci, and L. M. K. Vandersypen, Nature **601**, 343 (2022).

[2] B. Paquelet Wuetz, M. P. Losert, S. Koelling, L. E. A. Stehouwer, A.-M. J. Zwerver, S. G. J. Philips, M. T. Mądzik, X. Xue, G. Zheng, M. Lodari, S. V. Amitonov, N. Samkharadze, A. Sammak, L. M. K. Vandersypen, R. Rahman, S. N. Coppersmith, O. Moutanabbir, M. Friesen, and G. Scappucci, Nature Communications **13**, 7730 (2022).

[3] J. P. Dismukes, L. Ekstrom, and R. J. Paff, The Journal of Physical Chemistry **68**, 3021 (1964).

[4] O. Dyck, D. N. Leonard, L. F. Edge, C. A. Jackson, E. J. Pritchett, P. W. Deelman, and J. D. Poplawsky, Advanced Materials Interfaces **4**, 1700622 (2017).

[5] F. Pezzoli, E. Bonera, E. Grilli, M. Guzzi, S. Sanguinetti, D. Chrastina, G. Isella, H. Von Känel, E. Wintersberger, J. Stangl, and G. Bauer, Journal of Applied Physics **103**, 093521 (2008).

[6] F. Cerdeira, C. J. Buchenauer, F. H. Pollak, and M. Cardona, Physical Review B **5**, 580 (1972).

[7] L. H. Wong, C. C. Wong, J. P. Liu, D. K. Sohn, L. Chan, L. C. Hsia, H. Zang, Z. H. Ni, and Z. X. Shen, Japanese Journal of Applied Physics **44**, 7922 (2005).

[8] E. J. Connors, J. Nelson, H. Qiao, L. F. Edge, and J. M. Nichol, Physical Review B **100**, 165305 (2019).

[9] J. Dodson, H. E. Ercan, J. Corrigan, M. P. Losert, N. Holman, T. McJunkin, L. Edge, M. Friesen, S. Coppersmith, and M. Eriksson, Physical Review Letters **128**, 146802 (2022).

[10] B. L. Welch, Biometrika **34**, 28 (1947).
